# Supplementary material for: Adaptive and Dynamic Multi-Resolution Hashing for Pairwise Summations
Source: arXiv:2212.11408 source file (2022-12-21)
Supplement: Supplementary file 1 [file appendix.tex]

We first present probability tools in Section~\ref{sec:tools}.
We present the dynamic single-resolution $\HBE$ data structure design and corresponding lemmas in Section~\ref{sec:dynamic_single_hbe_appendix}.
We then present the dynamic multi-resolution $\HBE$ data structure design and lemmas in Section~\ref{sec:dynamic_multi_hbe_appendix}.
We present the proofs for \textsc{InsertX} and \textsc{DeleteX} in Section~\ref{sec:missing_proofs}.

\section{Notations and Probability Tools}\label{sec:tools}

For a positive integer $n$, we use $[n]$ to denote set $\{1,2,\cdots, n\}$.  We use $\Pr[\cdot]$ to denote the probability, and use $\E[\cdot]$ to denote the expectation if it exists.

We will make use of Hoeffding's Inequality:
\begin{theorem}[\cite{blm13}]\label{them:hoeffding_inequality}
Let $X_{1}, \ldots, X_{n}$ be independent random variables such that $X_{i} \in[a_{i}, b_{i}]$ almost surely for $i \in[n]$ and let $S=\sum_{i=1}^{n} X_{i}-\mathbb{E}[X_{i}]$. Then, for every $t>0$ :
\begin{align*}
 \Pr[S \geq t] \leq \exp (-\frac{2 t^{2}}{\sum_{i=1}^{n}(b_{i}-a_{i})^{2}}) .
\end{align*}

\end{theorem}
